# Supplementary material for: Ultra-small moment incommensurate spin density wave order masking a ferromagnetic quantum critical point in NbFe$_2$
Source: arXiv:1704.08379 ancillary file (2019-08-29)
Supplement: Supplementary file 1 [file NbFe2_neutron_elastic_1704_submission_supplement.pdf]

# Ultra-small moment incommensurate spin density wave order masking a ferromagnetic quantum critical point in NbFe<sub>2</sub> - Supplemental Material

P. G. Niklowitz,<sup>1,\*</sup> M. Hirschberger,<sup>2</sup> M. Lucas,<sup>1</sup> P. Cermak,<sup>3</sup> A. Schneidewind,<sup>3</sup> E. Faulhaber,<sup>4</sup> J.-M. Mignot,<sup>5</sup> W. J. Duncan,<sup>1</sup> A. Neubauer,<sup>6</sup> C. Pfleiderer,<sup>6</sup> and F. M. Grosche<sup>7</sup>

<sup>1</sup>Department of Physics, Royal Holloway, University of London, Egham TW20 0EX, U.K.

<sup>2</sup>Department of Physics, Princeton University, Princeton, NJ08544, U.S.A.

<sup>3</sup>Jülich Centre for Neutron Science (JCNS) at Heinz Maier-Leibnitz Zentrum (MLZ), Forschungszentrum Jülich GmbH, Lichtenbergstr. 1, 85748 Garching, Germany

<sup>4</sup>Heinz Maier-Leibnitz Zentrum (MLZ), Technische Universität München, Lichtenbergstr. 1, 85748 Garching, Germany

<sup>5</sup>Laboratoire Léon Brillouin (CEA-CNRS), CEA Saclay, F-91191 Gif-sur-Yvette, France

<sup>6</sup>Physik Department E21, Technische Universität München, 85748 Garching, Germany

<sup>7</sup>Cavendish Laboratory, University of Cambridge, Cambridge CB3 0HE, U.K.

PACS numbers:

Keywords:

## SAMPLE CHARACTERISATION

We have studied three large single crystals, which are approximately 6 mm wide and between 4 and 15 mm long.

*Sample A* (designation OFZ12-x). In magnetic susceptibility measurements (Fig. 1) this sample shows a

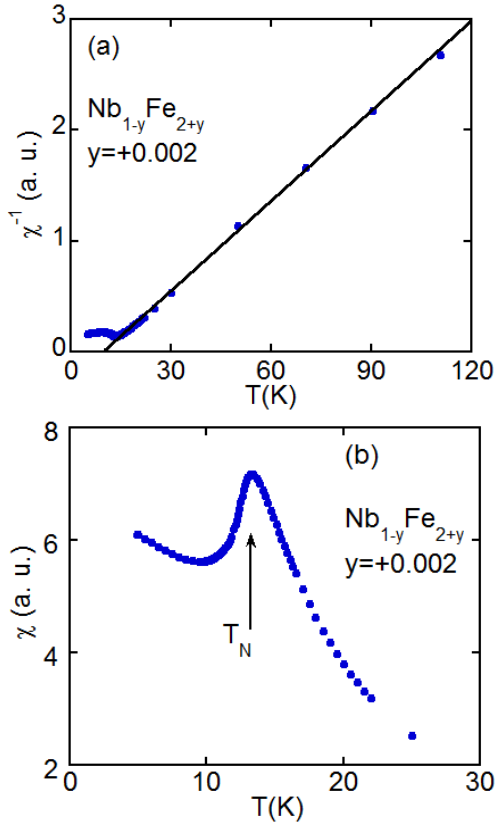

FIG. 1:  $T$  dependence of the magnetic susceptibility of Sample A. (a) shows the inverse susceptibility and (b) the low-temperature susceptibility, where  $T_N = 13$  K (arrow) is observed.

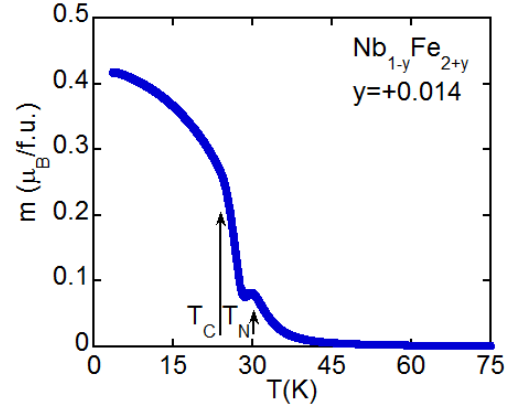

FIG. 2:  $T$  dependence of the magnetisation measured after field cooling of a piece cut off from Sample B.  $T_N$  and  $T_C$  are observed at 30 K and 24 K, respectively (arrows).

distinct peak at  $T_N = 13$  K and no ferromagnetism down to 2 K. The peak position agrees with the observed onset temperature of SDW order in our neutron data.

*Sample B* (designation OFZ27.3). In our magnetisation measurements (Fig. 2) a fragment cut from Sample B shows two phase transition anomalies, at  $T_C = 24$  K and  $T_N = 30$  K. The onset temperatures of Sample B in neutron scattering are  $T = 24.5$  K for the FM transition and  $T = 32.5$  K for the SDW transition (main text Fig. 3). We note that the peak intensity for the SDW signature in neutron scattering coincides with the FM onset temperature of  $T = 24.5$  K, whereas the SDW intensity vanishes at  $T = 19$  K. Because we know from prior magnetic studies that the SDW-FM transition is first order, this overlap region of 5.5 K must be attributed to a distribution of sample compositions. Main text Fig. 1 shows that a variation of  $T_C$  by  $\pm 2.8$  K corresponds to a variation of composition  $y$  by  $\pm 0.0016$ . This composition variation leads, in turn, to a variation of  $T_N$  by  $\pm 2.2$  K. This causes the *bulk* neutron transition tem-

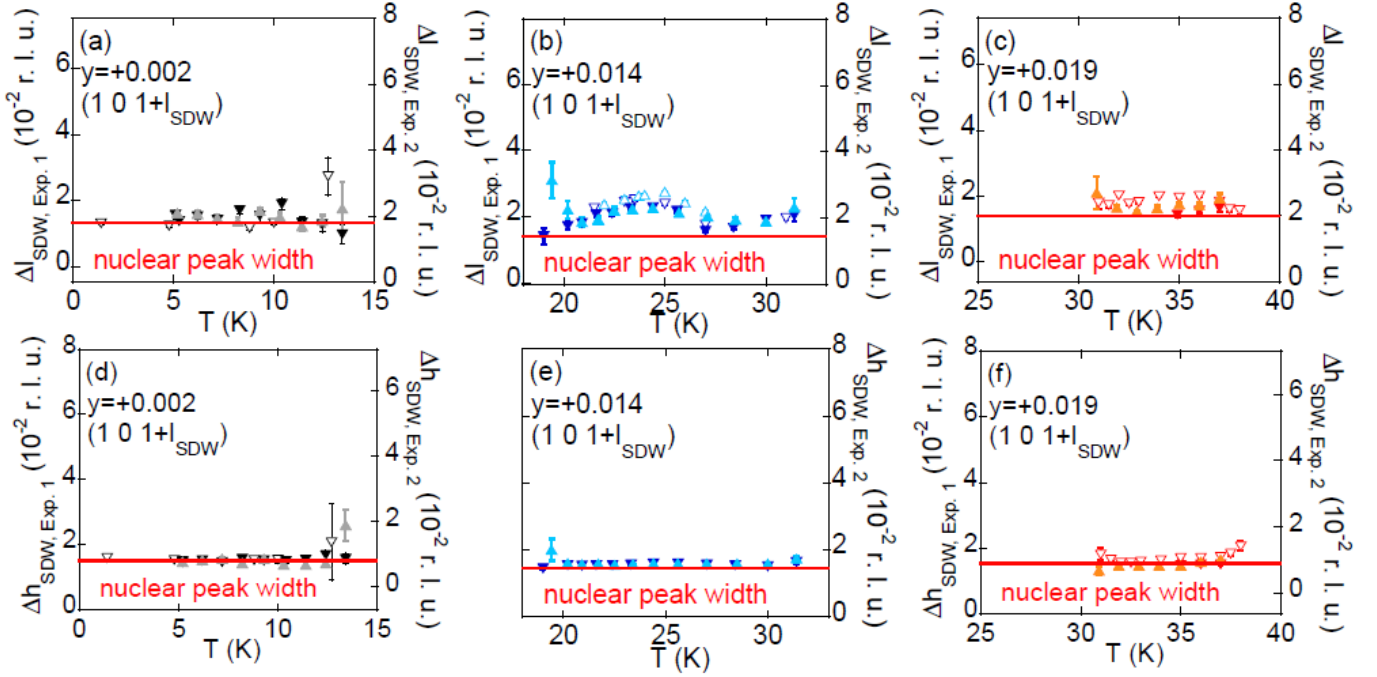

FIG. 3: Neutron diffraction at  $\mathbf{Q} = (1, 0, 1+l_{\text{SDW}})$  of  $\text{Nb}_{1-y}\text{Fe}_{2+y}$  samples A ( $y = +0.002$ ), B ( $y = +0.014$ ), and C ( $y = +0.019$ ). The  $T$  dependence of the SDW peaks'  $l$  and  $h$  widths is shown in Figures (a)-(c) and (d)-(f), respectively. SDW peak width values are weighted average widths whenever multiple Gaussian fit functions have been used. The SDW peak widths are compared to the corresponding width values of the nearby nuclear (101) peaks, which are indicated by red lines and have been obtained by equivalent Gaussian fits.

peratures to be about 2.8 K (2.3 K) lower than the onset temperatures for  $T_C$  ( $T_N$ ), respectively, and gives  $T_{C,\text{neutrons,bulk}} \approx 21.7$  K and  $T_{N,\text{neutrons,bulk}} \approx 30.2$  K, in good agreement with the magnetisation data shown in Fig. 2. Moreover, neutron depolarisation measurements of Sample B have previously suggested a FM onset temperature between  $T = 24$  K and  $T = 26$  K (Ref. [1]) and confirmed homogeneous FM order below  $T = 19$  K, where our neutron diffraction data shows that SDW order is fully suppressed.

*Sample C* (designation OFZ28.3.2.4). Prior AC susceptibility and magnetisation measurements on a fragment cut from this large crystal (Ref. [2]) show two phase transition anomalies, at  $T_C = 33$  K and  $T_N = 37$  K. The onset temperatures in our neutron data (main text Fig. 3) are  $T = 34.5$  K for the FM transition and  $T = 38$  K for the SDW transition. The SDW/FM overlap region (main text Fig. 3b) is about 4 K wide, suggesting that the bulk transition temperatures fall 2 K (1.6 K) below the onset temperatures for FM (SDW), respectively. This gives  $T_{C,\text{neutrons,bulk}} \approx 32.5$  K and  $T_{N,\text{neutrons,bulk}} \approx 36.4$  K, in good agreement with the magnetic measurements in Ref. [2]. Neutron depolarisation measurements at temperatures of up to  $T = 30$  K have confirmed a homogeneous FM state [1].

## EXPERIMENTAL SET-UP

Neutron diffraction was carried out at two cold triple-axis spectrometers in diffraction mode: Panda operated by JCMS at the Heinz Maier-Leibnitz Zentrum (MLZ) and 4F2 at the Laboratoire Léon Brillouin (LLB). At both instruments both PG monochromator and PG analyser were set to be vertically focusing and horizontally flat. No collimation was used. Higher-order harmonics were removed from the scattered beam by a closed-cycle refrigerator cooled Be filter after the sample and monitor correction for higher order neutrons has been included in the analysis.

## DATA ANALYSIS

For the analysis of the SDW Bragg reflections the shape of the fit function has been determined by the shape of the nearby nuclear (101) Bragg reflection, which is influenced by sample mosaicity and instrumental resolution. In all cases  $\mathbf{q}$  scans through (101) revealed single, double, or triple Gaussian peak shapes. The resulting nuclear peak shape has then been used to fit the SDW Bragg reflections. The SDW peak fit functions also contain a constant background contribution. In the case of Sample C the background also contains contributions from a

weak broad Gaussian centred at  $\mathbf{q}_{\text{SDW}}$ , and from a very weak Gaussian tail of the nuclear (101) Bragg reflection.

In order to obtain the  $T$  dependence of the integrated intensities of the FM Bragg reflections, the  $T$  dependence of the (102) count rates have been measured and a linear nuclear background has been subtracted.

### SDW BRAGG PEAK WIDTHS

The SDW and nuclear peak widths are generally found to be very similar. The  $l$  and  $h$  widths of the SDW Bragg reflection at  $\mathbf{Q} = (1, 0, 1 + l_{\text{SDW}})$  are shown in Fig. 3. The widths are compared to the corresponding width values of the nearest nuclear (101) Bragg reflection. Only in the range where  $\mathbf{q}_{\text{SDW}}$  is  $T$  dependent SDW Bragg peaks show slight broadening in the  $l$  direction corresponding to a correlation length of the order of 100 nm, which is otherwise found to be at least of the order of  $1 \mu\text{m}$ .

### ESTIMATE OF THE SDW ORDERED MOMENT

Absolute estimates of the SDW ordered moment are made by comparing the integrated intensities of the SDW Bragg peaks to the FM Bragg peak intensity in Sample C. Integrated intensities of the FM Bragg peak have been obtained from the FM peak intensities by assuming that nuclear and FM signal widths are similar. In order to carry out the comparison between SDW and

FM intensities, it has been assumed that both the ordered SDW and FM moments point along the easy  $c$ -axis. The FM intensities have then been multiplied with a correction factor of 1.26 to account for the stronger selection-rule effect at  $\mathbf{Q} = (1, 0, 2)$  compared to  $\mathbf{Q} = (1, 0, 1 + l_{\text{SDW}})$ . The correspondence between integrated FM Bragg peak intensities and the sizes of the ordered moment is fixed at  $T = 13 \text{ K}$ , where the ordered moment of the piece cut off from Sample C has been independently determined by DC magnetisation measurements to be  $\mu = 0.12 \mu_{\text{B}}/(\text{Fe atom})$  [2]. This leads to estimated upper bounds for the maximum ordered SDW moments in the three studied samples in the range from  $\mu_{\text{s}} = 0.03 \mu_{\text{B}}/(\text{Fe atom})$  to  $\mu_{\text{s}} = 0.08 \mu_{\text{B}}/(\text{Fe atom})$ , although these values could be reduced with the inclusion of extinction effects and domain formation on the FM signal. Domain effects might also lead to an observed variation by up to a factor 2 in the size of the ordered SDW moment obtained from the analysis of different measurements of the same sample.

---

\* e-mail: [philipp.niklowitz@rhul.ac.uk](mailto:philipp.niklowitz@rhul.ac.uk)

- [1] A. Neubauer, Ph.D. thesis, Technische Universität München (2011).
- [2] T. D. Haynes, I. Maskery, M. W. Butchers, J. A. Duffy, J. W. Taylor, S. R. Giblin, C. Utfeld, J. Laverock, S. B. Dugdale, Y. Sakurai, et al., Phys. Rev. B **85**, 115137 (2012).
